# Supplementary material for: Generation of Tin-Vacancy Centers in Diamond via Shallow Ion Implantation and Subsequent Diamond Overgrowth
Source: arXiv:1910.14165 source file (2020-02-19)
Supplement: Supplementary file 1 [file supporting_information.pdf]

# Supporting Information for Generation of Tin-Vacancy Centers in Diamond via Shallow Ion Implantation and Subsequent Diamond Overgrowth

Alison E. Rugar,*,† Haiyu Lu,‡,§ Constantin Dory,† Shuo Sun,† Patrick J. McQuade,¶,‖ Zhi-Xun Shen,‡,‖ Nicholas A. Melosh,¶,‖ and Jelena Vučković†

†*E. L. Ginzton Laboratory, Stanford University, Stanford, California 94305, United States*

‡*Department of Physics, Stanford University, Stanford, California 94305, United States*

¶*Department of Materials Science and Engineering, Stanford University, Stanford, California 94305, United States*

§*Geballe Laboratory for Advanced Materials, Stanford University, Stanford, California 94305, United States*

‖*Stanford Institute for Materials and Energy Sciences, SLAC National Accelerator Laboratory, Menlo Park, California 94025, United States*

E-mail: arugar@stanford.edu

## Photoluminescence measurements

For all PL measurements, we used a home-built scanning confocal microscope with a 0.9-NA objective. A diode laser with a central wavelength of 520 nm was used for excitation. The excitation light was spectrally filtered by a 550-nm short-pass (550SP) filter.

For the PL spectra shown in Figures 2 and 3 of the main text, the detected light was sent through a 568-nm long-pass (568LP) filter and a 594LP filter before being collected into a multimode fiber. The spectra are averages over three different spots on each of the samples. The 2D PL map and PL spectrum shown in Figure 4 of the main text was collected into a single-mode fiber after passing through 568LP and 594LP filters as well as a bandpass filter centered at 620 nm with a bandwidth of 14 nm (620/14).

# Probing the origin of the peak at P2

We explore whether the peak at P2 is a feature of the phonon sideband of the $SnV^-$ center or a separate color center by comparing the spectra collected for two different excitation wavelengths: 520 nm and 632.8 nm (HeNe laser). The resulting spectra are presented in Figure S1. The spectra were taken with the setup described in the previous section for Figures 2 and 3, changing only the filters. For the 632.8-nm excitation, a 632.8-nm laser clean-up filter was used in the excitation path and the collected light passed through 550LP and 638LP filters before being coupled into a multimode fiber.

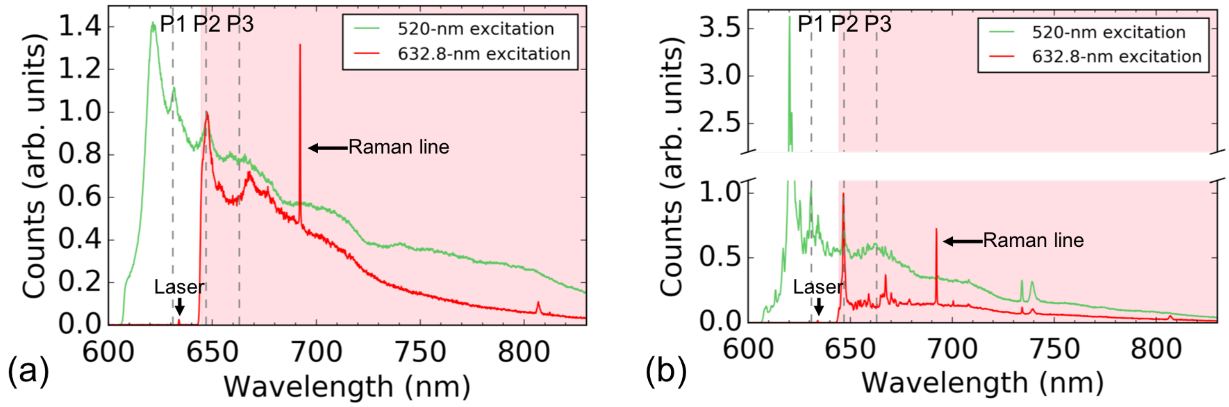


Figure S1: Comparing the bulk spectra collected from sample A for two different excitation wavelengths at (a) room temperature and (b) 5 K. Spectra are averaged over three different spots on sample A. The narrow peak at 691 nm is the diamond Raman line excited by HeNe laser light. The pink shaded region indicates the wavelengths for which the 638LP transmission exceeds 90%.

With both excitation wavelengths, the 647-nm line is apparent. The spectra presented

in Figure S1 are normalized to the maximum value on each of the 647-nm peaks. Because 632.8 nm is a longer wavelength than that of the ZPL of the $SnV^-$ center, we would not expect to excite the $SnV^-$ center and thus would not expect to observe any emission from the $SnV^-$ center. The presence of the 647-nm line under 632.8-nm excitation therefore indicates that the 647-nm line is not from the phonon sideband of the $SnV^-$ but rather may be from another Sn-related[1] color center. Furthermore the spectra at wavelengths longer than 647 nm also differ significantly between the two excitation wavelengths. For example, the spectrum taken with 632.8-nm excitation no longer displays a bump around P3 but rather a dip. Another peak appears at a slightly longer wavelength than P3, around 668 nm.

# Inhomogeneous broadening

Sample C, characterized in Figure 3(c) of the main text, underwent an initial $O_2$ plasma etch of 6 $\mu$m and was subsequently implanted with $^{120}Sn^+$ with a dose of $2 \times 10^{11}$ cm$^{-2}$. Sample C was not patterned prior to implantation. The preparation of sample C is summarized in Table S1.

Table S1: Summary of the fabrication steps performed on the additional sample studied.

| **Sample** | **Pre-implantation steps** | **Implantation conditions** | **Post-implantation steps** |
|---|---|---|---|
| C | tri-acid clean, 6 $\mu$m $O_2$ plasma etch | 1 keV, $2 \times 10^{11}$ cm$^{-2}$ | $H_2$ plasma clean, 90 nm MPCVD diamond growth |

Fits to the data presented in Figure 3 of the main text were found with the SciPy function `curve_fit` in Python. The curves were fit to a sum of three Gaussians. Two Gaussians fit the C and D transitions. The full widths at half-maxima were extracted from those two Gaussians. The third Gaussian fit a broader Gaussian background.

# Conversion efficiency estimate

We estimate the conversion efficiency by measuring the PL spectra at each of the 120 sites of the holes in the array shown in Figure 4 of the main text. From each spectrum we count how many $SnV^-$ ZPLs are present. At 5 K, only two ZPLs can be observed for a single $SnV^-$ center.[2] Thus, by counting pairs of distinct peaks around 620 nm, we obtain a rough estimate of a lower bound on the number of $SnV^-$ centers present in the spot under study. This approach leads to an underestimate of how many distinct $SnV^-$ centers are present at a particular spot because the ZPLs from multiple $SnV^-$ centers can overlap.

We compute how many ions were implanted per site in the array by multiplying implantation dose by the area exposed through the holes, assuming the holes to be 30 nm$\times$30 nm, as designed. Dividing the underestimate of $SnV^-$ centers present in the array by the expected number of implanted ions, we find an estimated lower bound on the conversion efficiency to be 1%.

# References


(1) Tchernij, S. D.; Herzig, T.; Forneris, J.; Küpper, J.; Pezzagna, S.; Train, P.; Morev, E.; Brida, I. P. D. G.; Skukan, N.; Genovese, M.; Jakšić, M.; Meijer, J.; Olivero, P. Single-Photon-Emitting Optical Centers in Diamond Fabricated upon Sn Implantation. *ACS Photonics* **2017**, *4*, 2580–6.

(2) Iwasaki, T.; Miyamoto, Y.; Taniguchi, T.; Siyushev, P.; Metsch, M. H.; Jelezko, F.; Hatano, M. Tin-Vacancy Quantum Emitters in Diamond. *Phys. Rev. Lett.* **2017**, *119*, 253601.
